# Supplementary material for: SHIELD: Suppressing Hallucinations In LVLM Encoders via Bias and Vulnerability Defense
Source: arXiv:2510.16596 source file (2026-02-10)
Supplement: Supplementary file 1 [file params.tex]

\begin{table}[ht]
% \small
\caption{Hyper-Parameters Setting}
\centering
\begin{tabular}{ccccc}
\toprule
Dataset                      & Param               & LLaVA-1.5     & InstructBLIP & Qwen-VL \\ \hline
\multirow{4}{*}{CHAIR}       & $\alpha$            & 2.0       & 0.5          & 3.0     \\
                             & $\beta$             & 0.35      & 0.8          & 0.5     \\
                             & $\varepsilon$       & 0.002     & 0.0          & 0.0     \\
                             & $K$                 & 32        & N/A          & 16      \\ \hline
\multirow{4}{*}{LLaVA Bench} & $\alpha$            & 2.0       & 0.5          & 3.0     \\
                             & $\beta$             & 0.55      & 0.8          & 0.5     \\
                             & $\varepsilon$       & 0.002     & 0.0          & 0.0     \\
                             & $K$                 & 32        & N/A          & 16      \\ \hline
\multirow{4}{*}{POPE} & $\alpha$                   & 1.64      & 2.8          & 4.0     \\
                             & $\beta$             & 0.2       & 0.55         & 0.06    \\
                             & $\varepsilon$       & 0.011     & 0.0          & 0.0     \\
                             & $K$                 & 32        & N/A          & 16      \\ \hline
\multirow{4}{*}{MME}         & $\alpha$            & 0.5       & 0.4          & 1.1     \\
                             & $\beta$             & 0.5       & 0.05         & 0.08    \\
                             & $\varepsilon$       & 0.004     & 0.0          & 0.0     \\
                             & $K$                 & 32        & N/A          & 16      \\ \bottomrule
\end{tabular}
\label{tab:hyparam}
\end{table}

% \begin{table}[ht]
% % \small
% \caption{Hyper-Parameters Setting}
% \centering
% \begin{tabular}{cccc}
% \toprule
% Param               & LLaVA-1.5      & InstructBLIP & Qwen-VL \\ \hline
% $\alpha$            & 2.0       & 0.5          & 3.0     \\
% $\beta$             & 0.35      & 0.8          & 0.5     \\
% $\varepsilon$       & 0.002     & 0.0          & 0.0     \\
% $K$                 & 32        & N/A          & 16      \\
% \bottomrule
% \end{tabular}
% \label{tab:hyparam}
% \end{table}

\section{Hyper-Parameters Setting}
During the experiments, we empirically tuned $\alpha$, $\beta$, $\varepsilon$, and $K$ for each VLM. Detailed parameter configurations are provided in the Table \ref{tab:hyparam}. Notably, InstructBLIP applies layer norm operations after the visual encoder to facilitate cross-modal interaction in Qformer, which partially alleviates inherent bias. Therefore, noise-derived visual tokens were not used to counter inherent biases on InstructBLIP.
