# Supplementary material for: SHIELD: Suppressing Hallucinations In LVLM Encoders via Bias and Vulnerability Defense
Source: arXiv:2510.16596 source file (2026-02-10)
Supplement: Supplementary file 3 [file K-ablation.tex]

\begin{table}[]
\centering
\begin{tabular}{c|cc}
\toprule
$K$    & CHAIR-S$\downarrow$       & CHAIR-I$\downarrow$      \\ 
\hline
8          & 39.6                      & 11.3          \\
16         & 38.2                      & 10.28\\
32         & \textbf{36.6}             & \textbf{10.3} \\
64         & 38.4                      & 11.5          \\ 
\bottomrule
\end{tabular}
\caption{Ablation Studies of $K$ on CHAIR}
\label{tab:K-ablation}
\end{table}
