# Supplementary material for: SHIELD: Suppressing Hallucinations In LVLM Encoders via Bias and Vulnerability Defense
Source: arXiv:2510.16596 source file (2026-02-10)
Supplement: Supplementary file 4 [file LR-ablation.tex]

\begin{table}[]
\centering
\begin{tabular}{c|cc}
\toprule
Learning Rate    & CHAIR-S$\downarrow$       & CHAIR-I$\downarrow$      \\ 
\hline
0.01         & 37.8                      & 11.2          \\
0.02         & \textbf{36.6}             & \textbf{10.3} \\
0.03         & 38.0                      & 11.2          \\
0.04         & 43.2                      & 11.6          \\ 
\bottomrule
\end{tabular}
\caption{Ablation Studies of Learning Rate on CHAIR}
\label{tab:lr-ablation}
\end{table}
