# Supplementary material for: SHIELD: Suppressing Hallucinations In LVLM Encoders via Bias and Vulnerability Defense
Source: arXiv:2510.16596 source file (2026-02-10)
Supplement: Supplementary file 5 [file alpha-ablation.tex]

\begin{table}[]
\centering
\begin{tabular}{c|cc}
\toprule
$\alpha$    & CHAIR-S$\downarrow$       & CHAIR-I$\downarrow$      \\ 
\hline
1.0         & 41.6                      & 11.6          \\
1.5         & 40.2                      & 11.2          \\
2.0         & \textbf{36.6}             & \textbf{10.3} \\
2.5         & 38.4                      & 10.7          \\ 
\bottomrule
\end{tabular}
\caption{Ablation Studies of $\alpha$ on CHAIR}
\label{tab:alpha-ablation}
\end{table}
