# Supplementary material for: SHIELD: Suppressing Hallucinations In LVLM Encoders via Bias and Vulnerability Defense
Source: arXiv:2510.16596 source file (2026-02-10)
Supplement: Supplementary file 6 [file beta-ablation.tex]

\begin{table}[]
\centering
\begin{tabular}{c|cc}
\toprule
$\beta$    & CHAIR-S$\downarrow$       & CHAIR-I$\downarrow$      \\ 
\hline
0.20         & 36.8                      & 11.2          \\
0.25         & 38.0                      & 11.0          \\
0.30         & \textbf{36.2}             & \textbf{10.3} \\
0.35         & 36.6                      & 10.3          \\ 
\bottomrule
\end{tabular}
\caption{Ablation Studies of $\beta$ on CHAIR}
\label{tab:beta-ablation}
\end{table}
