# Supplementary material for: SHIELD: Suppressing Hallucinations In LVLM Encoders via Bias and Vulnerability Defense
Source: arXiv:2510.16596 source file (2026-02-10)
Supplement: Supplementary file 7 [file infer_overhead.tex]

\begin{table}[t]
\scriptsize
\centering
\caption{Inference Overhead on POPE COCO using LLaVA-1.5}
\begin{tabular}{ccccc}
\hline
Method     & Accuracy $\uparrow$      & F1 $\uparrow$           & Time/Sample (ms) $\downarrow$  & Relative $\downarrow$        \\ \hline
Vanilla    & 81.3                     & 79.6                    & \textbf{128}      & \textbf{1.0×}   \\
VCD        & 84.6                     & 84.4                    & 190               & 1.5×            \\
OPERA      & 84.7                     & 85.4                    & 1586              & 12.4×            \\
\rowcolor[HTML]{C0C0C0} 
Ours & \textbf{87.0}            & \textbf{87.4}           & 980               & 7.6×            \\ \hline
\end{tabular}
\label{tab:infer-overhead}
\end{table}
