# Supplementary material for: SHIELD: Suppressing Hallucinations In LVLM Encoders via Bias and Vulnerability Defense
Source: arXiv:2510.16596 source file (2026-02-10)
Supplement: Supplementary file 8 [file unify-params.tex]

% Please add the following required packages to your document preamble:
% \usepackage{multirow}
% \usepackage[table,xcdraw]{xcolor}
% Beamer presentation requires \usepackage{colortbl} instead of \usepackage[table,xcdraw]{xcolor}
\begin{table}[h]
\caption{Comparison with training-free methods using a unified hyperparameter setting. Results are obtained using the same default configuration (\(\alpha=2\), \(\beta=0.35\), \(\varepsilon=0\), \(K=32\)) across all datasets.}
\begin{tabular}{ccccccc}
\toprule
                         & \multicolumn{2}{c}{POPE}          & \multicolumn{2}{c}{MME}               & \multicolumn{2}{c}{CHAIR} \\ \cline{2-7} 
\multirow{-2}{*}{Method} & Avg Acc$\uparrow$ & Avg F1$\uparrow$ & Hal$\uparrow$ & Full$\uparrow$ & $C_S$ $\downarrow$ & $C_I$ $\downarrow$ \\ \hline
Vanilla                  & 81.3              & 79.6          & 565.3                      & 1632.1   & 48.8        & 14.2        \\
VCD                      & 84.6              & 84.4          & 604.6                      & 1717.1   & 46.8        & 13.2        \\
OPERA                    & 84.7              & 85.4          & 592.3                      & 1717.2   & 44.6        & 12.8        \\
\rowcolor[HTML]{C0C0C0} 
Ours                     & \textbf{86.5}              & \textbf{86.1}          & \textbf{621.6}                      & \textbf{1737.1}   & \textbf{43.4}        & \textbf{11.7}        \\ \bottomrule
\end{tabular}
\label{tab:unify-params}
\end{table}
