# Supplementary material for: SHIELD: Suppressing Hallucinations In LVLM Encoders via Bias and Vulnerability Defense
Source: arXiv:2510.16596 source file (2026-02-10)
Supplement: Supplementary file 9 [file varepsilon-ablation.tex]

\begin{table}[]
\centering
\begin{tabular}{c|cc}
\toprule
$\varepsilon$   & CHAIR-S$\downarrow$       & CHAIR-I$\downarrow$      \\ 
\hline
0.000           & 38.8                      & 10.9          \\
0.002           & \textbf{36.6}             & \textbf{10.3} \\
0.004           & 37.0                      & 11.3          \\
0.006           & 39.4                      & 11.8          \\ 
\bottomrule
\end{tabular}
\caption{Ablation Studies of $\varepsilon$ on CHAIR}
\label{tab:varepsilon-ablation}
\end{table}
