# Supplementary material for: SHIELD: Suppressing Hallucinations In LVLM Encoders via Bias and Vulnerability Defense
Source: arXiv:2510.16596 source file (2026-02-10)
Supplement: Supplementary file 19 [file AttackStrategy.tex]

\begin{table}[h]
\centering
\scriptsize
\caption{Effect of Attack Strategy on CHAIR}
% {\color{blue}
\begin{tabular}{l|cc}
\toprule
Configuration & $C_S$~($\downarrow$) & $C_I$~($\downarrow$) \\
\midrule
Vanilla & 48.8 & 14.2 \\
Ours w/ FGSM-based Vulnerability Module & 39.2 & 11.5 \\
Ours w/ PGD-based Vulnerability Module & 37.2 & 11.3 \\
Ours (Learnable Attack) & \textbf{36.6} & \textbf{10.3} \\
\bottomrule
\end{tabular}
% }
\label{tab:attack-strategy}
\end{table}
