# Supplementary material for: SHIELD: Suppressing Hallucinations In LVLM Encoders via Bias and Vulnerability Defense
Source: arXiv:2510.16596 source file (2026-02-10)
Supplement: Supplementary file 26 [file MMhal.tex]

\begin{table}[htbp]
\centering
\scriptsize
\caption{GPT-4 Assisted Evaluation on MMHal-Bench}
\vspace{-4pt}
% {\color{blue}
\begin{tabular}{l|c|c|cccccccc}
\toprule
Method  & Overall~$\uparrow$ & Hallucination~$\downarrow$ & Attr.~$\uparrow$ & Adv.~$\uparrow$ & Comp.~$\uparrow$ & Cnt.~$\uparrow$ & Rel.~$\uparrow$ & Env.~$\uparrow$ & Hol.~$\uparrow$ & Other~$\uparrow$ \\
\midrule
Vanilla & 2.21 & 0.70 & \textbf{2.75} & \textbf{2.00} & 2.50 & 2.50 & 1.67 & 2.17 & 1.83 & 2.25 \\
Ours    & \textbf{2.65} & \textbf{0.61} & 2.42 & 1.83 & \textbf{2.58} & \textbf{2.67} & \textbf{2.83} & \textbf{3.92} & \textbf{2.08} & \textbf{2.83} \\
\bottomrule
\end{tabular}
% }
\label{tab:mmhal}
\vspace{-6pt}
\end{table}
