# Supplementary material for: SHIELD: Suppressing Hallucinations In LVLM Encoders via Bias and Vulnerability Defense
Source: arXiv:2510.16596 source file (2026-02-10)
Supplement: Supplementary file 33 [file params-ablation.tex]

\begin{table*}[h]
\scriptsize
\centering

\begin{minipage}{0.23\textwidth}
    \centering
    \caption{$\alpha$ Ablation}
    \begin{tabular}{c|cc}
    \toprule
    $\alpha$ & $C_S$$\downarrow$ & $C_I$$\downarrow$ \\ 
    \hline
    1.0 & 41.6 & 11.6 \\
    1.5 & 40.2 & 11.2 \\
    2.0 & \textbf{36.6} & \textbf{10.3} \\
    2.5 & 38.4 & 10.7 \\ 
    \bottomrule
    \end{tabular}
    \label{tab:alpha-ablation}
\end{minipage}%
\hspace{0.01\textwidth}
\begin{minipage}{0.23\textwidth}
    \centering
    
    \caption{$\beta$ Ablation}
    \begin{tabular}{c|cc}
    \toprule
    $\beta$ & $C_S$$\downarrow$ & $C_I$$\downarrow$ \\ 
    \hline
    0.20 & 36.8 & 11.2 \\
    0.25 & 38.0 & 11.0 \\
    0.30 & \textbf{36.2} & \textbf{10.3} \\
    0.35 & 36.6 & 10.3 \\ 
    \bottomrule
    \end{tabular}
    \label{tab:beta-ablation}
\end{minipage}%
\hspace{0.01\textwidth}
\begin{minipage}{0.23\textwidth}
    \centering
    \caption{$K$ Ablation}
    \begin{tabular}{c|cc}
    \toprule
    $K$ & $C_S$$\downarrow$ & $C_I$$\downarrow$ \\ 
    \hline
    8  & 39.6 & 11.3 \\
    16 & 38.2 & 10.8 \\
    32 & \textbf{36.6} & \textbf{10.3} \\
    64 & 38.4 & 11.5 \\ 
    \bottomrule
    \end{tabular}
    \label{tab:K-ablation}
\end{minipage}%
\hspace{0.01\textwidth}
\begin{minipage}{0.23\textwidth}
    \centering
    \caption{$l$ Ablation}
    \begin{tabular}{c|cc}
    \toprule
    $l$ & $C_S$$\downarrow$ & $C_I$$\downarrow$ \\ 
    \hline
    0.01 & 37.8 & 11.2 \\
    0.02 & \textbf{36.6} & \textbf{10.3} \\
    0.03 & 38.0 & 11.2 \\
    0.04 & 43.2 & 11.6 \\ 
    \bottomrule
    \end{tabular}
    \label{tab:lr-ablation}
\end{minipage}%

\end{table*}
