# Supplementary material for: SHIELD: Suppressing Hallucinations In LVLM Encoders via Bias and Vulnerability Defense
Source: arXiv:2510.16596 source file (2026-02-10)
Supplement: Supplementary file 35 [file qwenresults.tex]

\begin{table}[t]
\centering
\scriptsize
\caption{Extended Evaluation on Recent VLMs Variants (POPE COCO Adversarial Split)}
% {\color{blue}
\begin{tabular}{l|cc|cc|cc}
\toprule
\multirow{2}{*}{Method} & \multicolumn{2}{c|}{Qwen2-VL (7B)} & \multicolumn{2}{c|}{Qwen2.5-VL (7B)} & \multicolumn{2}{c}{Qwen3-VL (8B)} \\
                        & Accuracy~($\uparrow$) & F1 Score~($\uparrow$) & Accuracy~($\uparrow$) & F1 Score~($\uparrow$) & Accuracy~($\uparrow$) & F1 Score~($\uparrow$) \\
\midrule
Vanilla & 85.3 & 84.5 & 85.6 & 85.1 & 86.2 & 85.8 \\
Ours    & \textbf{86.1} & \textbf{85.4} & \textbf{86.8} & \textbf{86.0} & \textbf{87.4} & \textbf{86.6} \\
\bottomrule
\end{tabular}
% }
\label{tab:qwen-variants}
\end{table}
