# Supplementary material for: SHIELD: Suppressing Hallucinations In LVLM Encoders via Bias and Vulnerability Defense
Source: arXiv:2510.16596 source file (2026-02-10)
Supplement: Supplementary file 36 [file stepablation.tex]

\begin{wraptable}[6]{r}{1.8in}
\vspace{-18pt}
\centering
\scriptsize
\caption{Attack Steps Ablation}
\vspace{-6pt}
% {\color{blue}
\begin{tabular}{c|cc}
\toprule
Steps & $C_S$$\downarrow$ & $C_I$$\downarrow$ \\ 
\hline
15 & 40.8 & 11.6 \\
30 & \textbf{36.6} & \textbf{10.3} \\
45 & 36.6 & 10.4 \\
\bottomrule
\end{tabular}
% }
\label{tab:attack-steps-ablation}
\end{wraptable}
